# Supplementary material for: TexGen: Text-Guided 3D Texture Generation with Multi-view Sampling and Resampling
Source: arXiv:2408.01291 source file (2024-08-02)
Supplement: Supplementary file 1 [file X_suppl.tex]

\clearpage
\setcounter{page}{1}

\maketitlesupplementary

\input{algorithms/algorithm_1}

\section{Algorithm Details}
\label{sec:algo}
% % 
% Having the supplementary compiled together with the main paper means that:
% %  
% \begin{itemize}
% \item The supplementary can back-reference sections of the main paper, for example, we can refer to \cref{sec:intro};
% \item The main paper can forward reference sub-sections within the supplementary explicitly (e.g. referring to a particular experiment); 
% \item When submitted to arXiv, the supplementary will already included at the end of the paper.
% \end{itemize}
% % 
% To split the supplementary pages from the main paper, you can use \href{https://support.apple.com/en-ca/guide/preview/prvw11793/mac#:~:text=Delete%20a%20page%20from%20a,or%20choose%20Edit%20%3E%20Delete).}{Preview (on macOS)}, \href{https://www.adobe.com/acrobat/how-to/delete-pages-from-pdf.html#:~:text=Choose%20%E2%80%9CTools%E2%80%9D%20%3E%20%E2%80%9COrganize,or%20pages%20from%20the%20file.}{Adobe Acrobat} (on all OSs), as well as \href{https://superuser.com/questions/517986/is-it-possible-to-delete-some-pages-of-a-pdf-document}{command line tools}.

To better illustrate the working flow of our proposed method, we present the detailed algorithm in Alg.~\ref{alg:1}

\section{Derivation of Eq.~\ref{eqn:multi_cond}}

As discussed in Eq.~\ref{eqn:multi_cond} of Sec.~\ref{sec:t2gr}, we apply the classifier-free guidance (CFG) on noise estimation with two conditions: the textual prompt $c$ and the intermediate texture map $\hat{U}_{0,t}^i$. The original text guided diffusion model targets at learning $P(x_t|c)$ where $x_t$ denotes the noisy latent feature at time step $t$. Now we extend the target of the original diffusion model to $P(x_t^i|c, \hat{U}_{0,t}^N)$, which has an additional condition $\hat{U}_{0,t}^N$ to constrain the generated $x_t^i$ to be view-consistent. We assume $P(c|x_t^i, \hat{U}_{0,t}^N) = P(c|x_t^i)$. Following Bayes' theorem, $P(x_t^i|c, \hat{U}_{0,t}^N)$ can be reformulated as
\begin{equation}
P(x_t^i|c, \hat{U}_{0,t}^N) = \frac{P(x_t^i) P(c|x_t^i) P(\hat{U}_{0,t}^N|x_t^i)}{P(c, \hat{U}_{0,t}^N)}.
\label{eqn:bayes}
\end{equation}

By taking logarithm on both sides of the above equation, we get 
\begin{equation}
\begin{aligned}
\log(P(x_t^i|c, \hat{U}_{0,t}^N)) =& \log(P(x_t^i)) \\
& + \log(P(c|x_t^i)) + \log(P(\hat{U}_{0,t}^N|x_t^i))\\ 
& - log(P(c, \hat{U}_{0,t}^N)).
\label{eqn:log}
\end{aligned}
\end{equation}

As mentioned in~\cite{poole2022dreamfusion}, estimating $\epsilon_m(x_t^i)$ is related to predicting the score function $s_m(x_t^i)$ of the approximate
marginal distribution $P(x_t^i|c, \hat{U}_{0,t}^N)$, which can be formulated as:
\begin{equation}
s_m(x_t^i) = \nabla_{x_t^i}\log(P(x_t^i|c, \hat{U}_{0,t}^N)),
\label{eqn:score}
\end{equation}
\begin{equation}
\epsilon_m(x_t^i) = -\sigma_t s_m(x_t^i),
\label{eqn:Tweedie’s}
\end{equation}
where $\sigma_t$ is the standard deviation of the latent noise parameterized by denoising step $t$. The score function $\nabla_{x_t^i}\log(P(x_t^i|c, \hat{U}_{0,t}^N))$ can be further derived from Eq.~\ref{eqn:log} as:
\begin{equation}
\begin{aligned}
\nabla_{x_t^i}\log(P(x_t^i|c, \hat{U}_{0,t}^N)) =& \nabla_{x_t^i}\log(P(x_t^i)) \\
& + \nabla_{x_t^i}\log(P(c|x_t^i)) \\
& + \nabla_{x_t^i}\log(P(\hat{U}_{0,t}^N|x_t^i)),
\label{eqn:score_derive}
\end{aligned}
\end{equation}
with
\begin{equation}
\begin{aligned}
\nabla_{x_t^i}\log(P(c|x_t^i)) =& \nabla_{x_t^i}\log(P(x_t^i|c)) \\
&- \nabla_{x_t^i}\log(P(x_t^i)),
\label{eqn:score_derive_c}
\end{aligned}
\end{equation}
\begin{equation}
\begin{aligned}
\nabla_{x_t^i}\log(P(\hat{U}_{0,t}^N|x_t^i)) =& \nabla_{x_t^i}\log(P(x_t^i|\hat{U}_{0,t}^N))\\
&- \nabla_{x_t^i}\log(P(x_t^i)),
\label{eqn:score_derive_texture}
\end{aligned}
\end{equation}
which correspond to the terms in our multi-conditioned CFG in Eq.~\ref{eqn:multi_cond} as:
\begin{equation}
\epsilon_\theta(x_t^i|\varnothing) = -\sigma_t \nabla_{x_t^i}\log(P(x_t^i)),
\label{eqn:epsilon_empty}
\end{equation}
\begin{equation}
\begin{aligned}
\epsilon_\theta(x_t^i|c) - \epsilon_\theta(x_t^i|\varnothing) =& -\sigma_t (\nabla_{x_t^i}\log(P(x_t^i|c)) \\
&- \nabla_{x_t^i}\log(P(x_t^i))),
\label{eqn:epsilon_text}
\end{aligned}
\end{equation}
\begin{equation}
\begin{aligned}
\epsilon_{tex}(x_t^i|\hat{U}_{0,t}^N) - \epsilon_\theta(x_t^i|\varnothing) =& -\sigma_t (\nabla_{x_t^i}\log(P(x_t^i|\hat{U}_{0,t}^N)) \\
&- \nabla_{x_t^i}\log(P(x_t^i))).
\label{eqn:epsilon_texture}
\end{aligned}
\end{equation}

Following CFG~\cite{ho2022classifier}, we apply two guidance scales $\omega_1$ and $\omega_2$ on two guidance terms. Finally, we have the multi-conditioned CFG as:
\begin{equation}
\begin{aligned}
\epsilon_m(x_t^i) = &\epsilon_\theta(x_t^i|\varnothing)\\ 
&+ \omega_1 (\epsilon_\theta(x_t^i|c) - \epsilon_\theta(x_t^i|\varnothing))\\
&+\omega_2 (\epsilon_{tex}(x_t^i|\hat{U}_{0,t}^N) - \epsilon_\theta(x_t^i|\varnothing)).
\end{aligned}
\label{eqn:multi_cond_copy}
\end{equation}

\section{Additional Experiments}

\subsection{Inference Time}

\input{tables/inference_time}

In Tab.~\ref{tab:time}, we compare the inference time of our proposed method with that of baseline methods on a single NVIDIA Tesla V100 GPU. 
% It shows that the score distillation based approaches (Fantasia3D~\cite{chen2023fantasia3d} and ProlificDreamer~\cite{wang2023prolificdreamer}) need lengthy optimization to converge. Although our method is slower than the TEXTure~\cite{richardson2023texture} and Text2Tex~\cite{chen2023text2tex} (which is mainly because of the Key and Value substitution as in Eq.~\ref{eqn:inpainting_3} and Eq.~\ref{eqn:inpainting_4}, and the MLP optimization for inverse rendering), our texture generation quality is higher than these two, which demonstrates that our method is an ideal trade-off between the performance and the efficiency. 

\subsection{More Qualitative Evaluations}

More qualitative evaluations are shown in Fig.~\ref{fig:more_qua}, Fig.~\ref{fig:sup_qua_1}, and Fig.~\ref{fig:sup_qua_2}. 

% sds: ps5_controller, keg2, fire_hydrant, pumpkin, Francois

% direct: turtle, lion2, dresser2, statue3, shark % update later
\input{figures/more_qualitative}
\input{figures/sup_qualitative_1}
\input{figures/sup_qualitative_2}

% more results: apple, armor, fireplace, lantern2, refrigerator, shark, pottery, telephone, vending_machine, helmet

\section{User Study Details}

We develop a WIX-based web application for the user study. As shown in Fig.~\ref{fig:us}, for each video pair, participants are required to choose the video that best illustrates the given textual prompt with the highest quality. They should then click the rounded check-box below the selected video and proceed to the next video pair. Finally, we determine the user preferences by counting all user selections.
\input{figures/user_study}

\section{Data Description}

We present the details of our collected data in Tab.~\ref{tab:data_1}, Tab.~\ref{tab:data_2}, and Tab.~\ref{tab:data_3} with corresponding textual prompts.

\input{tables/data_description_1}
\input{tables/data_description_2}
\input{tables/data_description_3}
